# Supplementary material for: DecArena: Evaluating Large-Scale Decentralized Multi-Agent Collaboration
Source: arXiv:2611.15521 source file (2026-11-11)
Supplement: Supplementary file 1 [file 091appendix_graph.tex]

% !TEX root = paper.tex
%
% Graph Definition and Construction
% ---------------------------------
% Self-contained section describing the formal graph model used by
% Skill-Graph and the procedures used to instantiate concrete graphs
% from a skill corpus.

\section{Graph Construction}
\label{sec:graph}

We first state the graph model (\Cref{sec:graph:model}), then specify the two orthogonal degrees of freedom that generate concrete instances of that model: skill \emph{placement} (\Cref{sec:graph:placement}), which assigns the skill pool to nodes, and \emph{edge construction} (\Cref{sec:graph:edges}), which links nodes to one another. The two axes are independent and form a Cartesian product (\Cref{sec:graph:grid}) that we use throughout the experimental section. We close with implementation notes on determinism, complexity, and the diagnostic statistics we report for every instantiated graph (\Cref{sec:graph:impl}).

% ---------------------------------------------------------------- model
\subsection{Graph Definition}
\label{sec:graph:model}



\paragraph{Skills.}
Each skill $s_i \in \mathcal{S}$ is a structured record
$s_i = (\textsc{id}_i, \textsc{name}_i, \textsc{desc}_i,
\textsc{body}_i, \mathcal{T}_i)$ consisting of a unique identifier, a
short name, a natural-language description, an optional executable
body, and a (possibly empty) set of categorical metadata tags
$\mathcal{T}_i$. A fixed encoder $\phi : \mathcal{S} \to \mathbb{R}^d$
maps each skill to an $L_2$-normalized embedding
$\mathbf{e}_i = \phi(s_i)$; we write $E \in \mathbb{R}^{N \times d}$
for the embedding matrix with rows $\mathbf{e}_i$. The encoder is
shared across all agents and the embedding is the only summary of a
skill's content that is exposed outside its owning agent.

\paragraph{Skill graph.}
A \emph{skill graph} over $\mathcal{S}$ and $\mathcal{A}$ is a tuple
\[
G = \bigl(\mathcal{A},\, \mathcal{E},\, \pi,\, \mu\bigr),
\]
in which the four components encode, respectively, the agents, the
network that connects them, how skills are scattered across them, and
how each agent advertises its own expertise:
\begin{itemize}[leftmargin=1.2em,itemsep=0.2em,topsep=0.2em]
\item \textbf{Agents} $\mathcal{A}$ are the nodes of the network and
the units of ownership and computation; an agent observes only its
own owned skills and the profiles of its immediate neighbors.
\item \textbf{Edges} $\mathcal{E} \subseteq \mathcal{A} \times
\mathcal{A}$ are the inter-agent communication links along which
queries may be forwarded. We write
$\mathcal{N}(a) = \{a' : (a, a') \in \mathcal{E}\}$ for the
out-neighborhood of $a$ and $\deg(a) = |\mathcal{N}(a)|$ for its
out-degree. The set $\mathcal{E}$ is fixed at construction time.
\item \textbf{Placement} $\pi : \mathcal{S} \to \mathcal{A}$ assigns
each skill to exactly one agent. We write $\mathcal{S}_a =
\pi^{-1}(a)$ for the skill set owned by $a$ and $n_a = |\mathcal{S}_a|$
for its size. By construction $\{\mathcal{S}_a\}_{a \in \mathcal{A}}$
is a partition of $\mathcal{S}$: skills are scattered, not
replicated, so $\sum_a n_a = N$ and
$\mathcal{S}_a \cap \mathcal{S}_{a'} = \varnothing$ for $a \neq a'$.
\item \textbf{Profile} $\mu : \mathcal{A} \to \mathbb{R}^d$ is a
public summary of the skills an agent owns, defined as the
$L_2$-normalized mean of their embeddings:
\begin{equation}
\mu(a) \;=\;
\frac{\sum_{s \in \mathcal{S}_a} \phi(s)}
     {\bigl\|\sum_{s \in \mathcal{S}_a} \phi(s)\bigr\|_2 + \varepsilon},
\label{eq:profile}
\end{equation}
where $\varepsilon > 0$ guards against empty agents. The profile is
the only information $a$ shares with its neighbors about its
contents, and it is the score function that local greedy routers use
to choose the next hop.
\end{itemize}

\paragraph{Locality of knowledge.}
The disjointness of $\pi$ formalizes the central asymmetry of our
setting: at any moment, an agent $a$ knows the full embeddings
$\{\mathbf{e}_i : s_i \in \mathcal{S}_a\}$ of the skills it owns, and
only the $d$-dimensional profiles $\{\mu(a') : a' \in \mathcal{N}(a)\}$
of its immediate neighbors. It does not know which specific skills
those neighbors own, nor anything about agents beyond one hop.
Consequently, a query for skill $s$ is answerable by exactly one agent
$\pi(s)$, and any improvement in answer quality must come from
\emph{routing the query through the network} until it reaches that
agent -- not from redundant placement, broadcasting, or a shared
index.

\paragraph{Two design axes.}
The graph definition above intentionally separates two design choices that prior work on multi-agent communication often couples: \emph{which skills each agent owns} (the placement $\pi$) and \emph{which agents talk to which} (the edge set $\mathcal{E}$). The profile map $\mu$ is determined by $\pi$ via \Cref{eq:profile}, so $\pi$ and $\mathcal{E}$ are the two free parameters of the construction. The remainder of this section instantiates these axes independent constructive axes, we obtain a clean factorial design space
in which the contribution of each axis can be measured. Routing
protocols (greedy, flood, learned) are layered on top of this fixed
substrate and are described elsewhere in the paper; the present
section is concerned solely with constructing $G$.

% ------------------------------------------------------------ placement
\subsection{Skill Placement}
\label{sec:graph:placement}

Placement is a function $\pi$ that defines $\mathcal{S}_a$ for every
agent $a$. We implement five placement strategies; together they span
the relevant axes of placement design (semantic coherence, topical
coherence, load skew, and adversarial near-duplicate splitting). All
strategies take as input the embedding matrix $E$, the target agent
count $A$, an integer seed $\sigma$, and (where applicable) the skill
metadata records.

\paragraph{Random ($\pi_{\textsc{rnd}}$).}
A uniform baseline. Each skill is assigned independently:
$\pi(s_i) \sim \mathrm{Uniform}(\mathcal{A})$. Profiles $\mu(a)$ under
$\pi_{\textsc{rnd}}$ have low cohesion and approach $\mathbf{0}$ in
expectation, which makes profile-based routing degenerate and serves as
the lower bound for routing performance.

\paragraph{Semantic ($\pi_{\textsc{sem}}$).}
We run spherical $k$-means with $K = A$ on the rows of $E$ and assign
each skill to its cluster's agent. The clustering uses
$k$-means$++$ initialization on the cosine similarity kernel
$\langle \mathbf{e}_i, \mathbf{e}_j \rangle$, alternates assignment
$z_i \leftarrow \arg\max_c \langle \mathbf{e}_i, \mathbf{c}_c \rangle$
with cluster recomputation $\mathbf{c}_c \leftarrow \mathrm{normalize}
(\mathrm{mean}\{\mathbf{e}_i : z_i = c\})$, and terminates either upon
convergence or after $T$ iterations ($T = 20$ in our experiments). This
strategy maximizes intra-agent cohesion and gives each agent a sharp,
interpretable profile; we report the cohesion statistic
$\bar{c}(a) = \frac{1}{n_a} \sum_{s \in \mathcal{S}_a}
\langle \phi(s), \mu(a) \rangle$ for every constructed graph.

\paragraph{Metadata-tag ($\pi_{\textsc{tag}}$).}
When skills carry categorical tags
$\mathcal{T}_i \neq \varnothing$ (e.g., \texttt{category},
\texttt{domain}, or a path-prefix of \textsc{id}$_i$), we group skills
by their primary tag and bucket the resulting tags into agents. Let
$\mathcal{T} = \bigcup_i \mathcal{T}_i$ denote the set of observed
tags. We compute a tag centroid
$\mathbf{t}_t = \mathrm{normalize}(\mathrm{mean}\{\mathbf{e}_i :
t \in \mathcal{T}_i\})$ for each tag $t$ and run $k$-means on
$\{\mathbf{t}_t\}$ with $K = A$. Tags within a cluster are merged into
the same agent; skills with no usable tag are distributed
round-robin into the smallest agents. When the fraction of tagged
skills falls below $50\%$, $\pi_{\textsc{tag}}$ falls back to
$\pi_{\textsc{sem}}$, ensuring the strategy is always runnable. The
tag strategy preserves human-meaningful boundaries that a purely
embedding-based partition may cut across.

\paragraph{Power-law ($\pi_{\textsc{pl}}$).}
We sample agent capacities $\{n_a\}$ from a discrete Zipf distribution:
\begin{equation}
n_a \;\propto\; r_a^{-\alpha},
\qquad r_a \in \{1, \ldots, A\},
\label{eq:zipf}
\end{equation}
with shape parameter $\alpha = 1.5$ unless otherwise noted, then rescale
so $\sum_a n_a = N$. To keep hubs semantically coherent we initialize
with $\pi_{\textsc{sem}}$ and \emph{redistribute} skills to honor the
sampled capacities: skills are processed in order of cluster surplus,
each claimed by the agent with maximal profile similarity that still
has remaining capacity. This produces a few hub agents owning many
related skills and a long tail of small specialists, modeling
real-world capability marketplaces in which a small number of providers
service most demand.

\paragraph{Adversarial ($\pi_{\textsc{adv}}$).}
This placement is designed to defeat purely local routing. We start
from $\pi_{\textsc{sem}}$ and then deliberately split near-duplicates
across agents: for each skill $s_i$ we identify its top-$k$ semantic
neighbors $\mathcal{B}_k(i)$ and, whenever a neighbor lies in the same
cluster, reassign it uniformly at random to a different cluster. The
number of such moves is bounded by a target $M$ (default $M = N/50$).
Under $\pi_{\textsc{adv}}$ a query that semantically resembles skill
$s_i$ will frequently retrieve a near-duplicate $s_j$ at a different
agent, forcing the router to traverse at least one edge to recover the
correct expert.

% ---------------------------------------------------------------- edges
\subsection{Edge Construction}
\label{sec:graph:edges}

Once placement is fixed, profiles $\mu(a)$ are determined by
\Cref{eq:profile}. Edge construction selects $\mathcal{E}$ given the
profile matrix $P \in \mathbb{R}^{A \times d}$ with rows $\mu(a)$ and
(where applicable) the skill counts $\{n_a\}$. We implement four edge
families that span the standard structural regimes
(Erd\H{o}s--R\'enyi, $k$-NN, Watts--Strogatz, Barab\'asi--Albert).
Each family takes a target out-degree $\deg \in \mathbb{N}$ and returns
a list of neighbors $\mathcal{N}(a)$ for every agent.

\paragraph{Random ($\mathcal{E}_{\textsc{rnd}}$).}
Each agent samples $\deg$ neighbors uniformly without replacement from
$\mathcal{A} \setminus \{a\}$. This realizes a $k$-regular random
graph and serves as a structureless baseline against which
similarity-aware constructions are compared.

\paragraph{Semantic $k$-nearest-neighbor ($\mathcal{E}_{\textsc{knn}}$).}
For each agent $a$ we compute pairwise cosine similarity
$\langle \mu(a), \mu(a') \rangle$ for $a' \neq a$ and connect $a$ to
the top-$\deg$ most similar agents. This produces clustered, locally
dense graphs whose effective diameter scales with the cluster count;
it is the structural analogue of $\pi_{\textsc{sem}}$.

\paragraph{Small-world ($\mathcal{E}_{\textsc{sw}}$).}
We start from $\mathcal{E}_{\textsc{knn}}$ and add $r$ random
``long-range'' shortcuts per agent
(Watts--Strogatz~\cite{watts1998collective}). Each shortcut links $a$
to a uniformly sampled non-neighbor, so the resulting graph retains
high clustering coefficient while collapsing the average shortest path
to $O(\log A)$. In our experiments $r = 2$ unless otherwise noted.

\paragraph{Scale-free ($\mathcal{E}_{\textsc{ba}}$).}
A Barab\'asi--Albert preferential-attachment process
\cite{barabasi1999emergence}. We seed the graph with a clique on
$m + 1$ nodes (with $m = \deg$) and add the remaining nodes one at a
time; each new node attaches $m$ undirected edges, with attachment
probabilities proportional to a per-node weight $w(a)$. Two weight
schedules are supported:
\begin{equation}
w_{\textsc{deg}}(a) \;=\; \mathrm{deg}(a) + \epsilon,
\qquad
w_{\textsc{sk}}(a) \;=\; n_a,
\label{eq:ba-weights}
\end{equation}
yielding the canonical degree-driven scale-free regime
($w_{\textsc{deg}}$) or a placement-coupled variant in which agents
owning more skills attract more edges ($w_{\textsc{sk}}$). The latter
captures the empirically observed coupling between capability and
connectedness in software ecosystems and online marketplaces.

\paragraph{Hierarchical (fused).}
A fifth, fused construction combines placement and edges in a single
two-level procedure. We run $\pi_{\textsc{sem}}$ with $K = A$ to obtain
\emph{leaf} agents and their profiles $\{\mu(a)\}$, then run a second
$k$-means with $K = C$ on the leaf profiles to obtain $C$
\emph{coordinator} agents whose profile is the centroid of the leaves
they parent. Leaves carry the full skill mass; coordinators carry no
skills, only profiles and child pointers. Edges are: each leaf to its
parent coordinator; coordinators to one another in a clique. The
resulting graph is a tree of depth two augmented with a
coordinator-level clique; greedy routing on this graph requires at
most $O(\log A)$ hops at the cost of introducing a routing bottleneck
at the coordinator layer. We treat hierarchical as a single cell in
our experimental grid because placement and edges are not separable
without breaking the construction.

% ------------------------------------------------------------------ grid
\subsection{The Construction Grid}
\label{sec:graph:grid}

The placement axis (5 strategies) and edge axis (4 strategies) define a
$5 \times 4 = 20$-cell Cartesian product, plus one fused
hierarchical cell, for a total of \textbf{21 graph instantiations} per
corpus and seed (\Cref{tab:grid}). Every cell is a fully specified
$(\pi, \mathcal{E})$ pair and can be constructed from the same
$(E, A, \sigma)$ triple. We use this grid throughout the experimental
section to disentangle the contribution of placement from that of
edges and to identify which combinations are robust across queries.

\begin{table}[t]
\centering
\small
\caption{The 21-cell construction grid. Rows are placements, columns
are edge families. The hierarchical cell fuses both axes (denoted
\fbox{H}) and is included as a 21st instantiation rather than a row or
column.}
\label{tab:grid}
\begin{tabular}{lcccc}
\toprule
 & $\mathcal{E}_{\textsc{rnd}}$ & $\mathcal{E}_{\textsc{knn}}$
 & $\mathcal{E}_{\textsc{sw}}$ & $\mathcal{E}_{\textsc{ba}}$ \\
\midrule
$\pi_{\textsc{rnd}}$ & \checkmark & \checkmark & \checkmark & \checkmark \\
$\pi_{\textsc{sem}}$ & \checkmark & \checkmark & \checkmark & \checkmark \\
$\pi_{\textsc{tag}}$ & \checkmark & \checkmark & \checkmark & \checkmark \\
$\pi_{\textsc{pl}}$  & \checkmark & \checkmark & \checkmark & \checkmark \\
$\pi_{\textsc{adv}}$ & \checkmark & \checkmark & \checkmark & \checkmark \\
\midrule
\multicolumn{5}{c}{Hierarchical (fused): \fbox{H}} \\
\bottomrule
\end{tabular}
\end{table}

% ---------------------------------------------------- end-to-end pipeline
\subsection{End-to-End Construction Pipeline}
\label{sec:graph:pipeline}

\Cref{alg:build} summarizes the pipeline. Inputs are the skill corpus
$\mathcal{S}$, the encoder $\phi$, the agent count $A$, a target
degree $\deg$, a placement choice $\pi^\star$, an edge choice
$\mathcal{E}^\star$, and a seed $\sigma$. Outputs are a fully
specified skill graph $G$ together with the per-cell statistics we use
for diagnostics (\Cref{sec:graph:impl}).

\begin{figure}[t]
\hrule\vspace{2pt}
\textbf{Algorithm 1}\quad\textsc{BuildSkillGraph}
\hrule\vspace{4pt}
{\small\ttfamily\raggedright
\begin{tabbing}
xxx\=xxx\=xxx\=\kill
\textbf{Inputs:}\ $\mathcal{S}$, $\phi$, $A$, $\deg$, $\pi^\star$,
$\mathcal{E}^\star$, $\sigma$ \\[1pt]
\textbf{Output:}\ skill graph $G = (\mathcal{A}, \mathcal{E}, \pi, \mu)$
\\[3pt]
1.\ \> $E \leftarrow [\phi(s_1); \ldots; \phi(s_N)]$ \\
2.\ \> $\{\mathcal{S}_a\}_{a=1}^A \leftarrow \pi^\star(E, A,
\mathcal{S}, \sigma)$ \\
3.\ \> \textbf{for}\ $a = 1, \ldots, A$\ \textbf{do} \\
4.\ \> \> $\mu(a) \leftarrow$ \textsc{Normalize}(mean of
$\{\phi(s) : s \in \mathcal{S}_a\}$) \\
5.\ \> \textbf{end for} \\
6.\ \> $\{n_a\} \leftarrow \{|\mathcal{S}_a|\}$ \\
7.\ \> $\{\mathcal{N}(a)\} \leftarrow \mathcal{E}^\star(P, \deg, \{n_a\},
\sigma)$ \\
8.\ \> \textbf{return}\ $G$ with profiles $P$, neighbors
$\{\mathcal{N}(a)\}$, owned skills $\{\mathcal{S}_a\}$
\end{tabbing}}
\hrule
\label{alg:build}
\end{figure}

The hierarchical cell replaces lines 2--7 with the fused two-level
procedure described in \Cref{sec:graph:edges}, which constructs
coordinators and leaves jointly.

% ------------------------------------------------------------ properties
\subsection{Construction Properties}
\label{sec:graph:props}

Three properties of \Cref{alg:build} are worth stating explicitly, as
they justify the experimental design used elsewhere in the paper.

\paragraph{Determinism.}
Every randomized step (Zipf sampling, $k$-means$++$ initialization,
small-world shortcuts, BA partner sampling) consumes from a single
NumPy \texttt{Generator} seeded with $\sigma$. Given fixed inputs and
$\sigma$, \Cref{alg:build} returns bit-identical $G$. This determinism
is required for the per-cell ablation tables in our experiments to be
reproducible.

\paragraph{Disjointness.}
$\pi$ is a function (not a relation), so $\{\mathcal{S}_a\}$ is a
partition of $\mathcal{S}$. No skill is replicated; the $i$-th query
can be answered correctly only by $\pi(s_i^\star)$, where $s_i^\star$
is the ground-truth target skill. Hence any improvement in answer
quality must arise from improved \emph{routing}, not from increased
redundancy of placement.

\paragraph{Decoupling of placement and edges.}
$\mathcal{E}^\star$ depends on placement only through profiles $P$ and
counts $\{n_a\}$. In particular, $\mathcal{E}_{\textsc{rnd}}$ is
\emph{independent} of placement, so cells in the
$\mathcal{E}_{\textsc{rnd}}$ column isolate the contribution of
placement; cells in the $\pi_{\textsc{rnd}}$ row isolate the
contribution of edges (modulo low-cohesion profiles). The grid is
therefore a true factorial design.

\paragraph{Complexity.}
Let $D$ be the embedding dimension. Embedding is $O(N D)$.
$k$-means runs in $O(T A N D)$. Profile computation is $O(N D)$.
$\mathcal{E}_{\textsc{rnd}}$ is $O(A \deg)$;
$\mathcal{E}_{\textsc{knn}}$ and $\mathcal{E}_{\textsc{sw}}$ require an
$A \times A$ similarity matrix at $O(A^2 D)$;
$\mathcal{E}_{\textsc{ba}}$ is $O(A \deg)$ if neighbor masks are kept
sparse. For our default $(A, N, D) = (400, 78\,361, 768)$ the
dominant cost is $k$-means on the $N \times D$ embedding matrix.

% ------------------------------------------------------------- impl
\subsection{Implementation Notes and Diagnostics}
\label{sec:graph:impl}

\paragraph{Embeddings.}
We support two interchangeable encoders that both emit
$L_2$-normalized vectors: a TF-IDF embedder over $n$-grams of orders
$(1, 2)$ with vocabulary cap $50\,000$ and minimum document
frequency $2$, used for fast iteration; and the released
\textsc{SkillRouter} bi-encoder \cite{skillrouter2026} (\textsc{SR-Emb-0.6B},
$d = 1024$), used for the headline numbers. The two encoders share an
identical interface, so all 21 cells can be constructed under either
encoder without code changes.

\paragraph{Output format.}
Each constructed cell is materialized to disk as a JSON manifest
\texttt{graph.json} containing per-agent metadata (id, role,
neighbors, children, owned-skill identifiers) plus a directory tree
\texttt{agents/agent\_*/skills/*/SKILL.md} containing the full skill
records. The manifest is the only file required by the orchestration
runtime; the per-skill directory tree exists so that downstream
runtimes can serve the skill bodies as filesystem-resident artifacts.

\paragraph{Reported diagnostics.}
For every constructed cell we report:
\begin{itemize}[leftmargin=1.2em,itemsep=0.2em,topsep=0.2em]
\item Skills-per-agent distribution: $\min$, median, $p_{95}$,
$\max$, mean.
\item Out-degree distribution: $\min$, median, $p_{95}$, $\max$, mean.
\item \emph{Cohesion}
$\bar{c} = \mathbb{E}_a [ \mathbb{E}_{s \in \mathcal{S}_a}
\langle \phi(s), \mu(a) \rangle ]$, the mean cosine of every owned
skill to its agent's profile, summarizing how semantically tight the
partition is.
\item Coordinator count (zero except in the hierarchical cell).
\end{itemize}
These statistics are required for any cell to enter our experimental
tables; outlier cells (e.g.\ degenerate $\pi_{\textsc{rnd}}$ profiles
under $\mathcal{E}_{\textsc{knn}}$) are flagged automatically.

\paragraph{Default hyperparameters.}
Unless otherwise specified, all experiments use $A = 400$,
$\deg = 6$, $r = 2$ (small-world shortcuts), $\alpha = 1.5$ (Zipf),
$M = N/50$ (adversarial moves), $C = 8$ (coordinators), $T = 20$
($k$-means iterations), and seed $\sigma = 0$. The released code
exposes every parameter on the command line so that ablations can be
reproduced without modification.
